# Supplementary material for: Optimal Resource Allocation with Delay Guarantees for Network Slicing in Disaggregated RAN
Source: arXiv:2305.17321 source file (2023-06-05)
Supplement: Supplementary file 1 [file Appendix.tex]

\appendix
\subsection{First Example}

Let flow 1 be the foi (flow of interest).

\begin{equation}
    D_{e2e}^{f^{'sl,u}}=\frac{\sigma^{f^{'sl,u}}}{\min_{s\in\mathcal{S}}{\{R_{s}^{sl,u}-\rho_{s}^{y(f^{'sl,u})}\}}}+\sum_{s \in \mathcal{S}}\left(T_{s}+\frac{\sum_{f\in \mathcal{F}_{s}^{sl,u},f\neq f^{'}}{}^*\sigma_{s}^{f}}{R_{s}^{sl,u}}\right),
	\label{eq:de2e_demo}
\end{equation}

\noindent where

\begin{equation}
    {}^{*}\sigma^{f}_{s}=\sigma^{f}+\rho^{f}\sum_{s\in\mathcal{H}^f}T_{s},
    \label{eq:burst_app}
\end{equation}

\begin{table}[htb]
	\centering
\begin{threeparttable}
	\caption{Parameters}
   \label{Tab:ParametersExample}

	\begin{tabular}{|c|c|c|c|c|}
		\hline
		Parameter & $R$ (Mbps) & $T\tnote{1}$ ($\mu$s) &  $\phi$ & PD ($\mu$s) \\
		\hline
		node 1 (vDU) & 50 & 40.96 &  0.5 & 0 \\
		\hline
            node 2 (eth) & 100 & 40.96 &  0.25 & 0 \\
		\hline
		node 3 (ring) & 250 & 36.384 &  0.25 & 20 \\
		\hline
		node 4 (ring) & 250 & 28.192 &  0.125 & 20 \\
		\hline
		node 5 (ring) & 250 & 24.096 &  0.0625 & 20 \\
            \hline
		\hline
		Parameter & $\rho$ (bps) & $\sigma$ (bits) &  pkt size (Bytes) & Use case \\
            \hline
		flow 1  & $1024\times 10^3$ & 1024 &  128 & URLLC \\
		\hline
		flow 2  & $512\times 10^3$ & 4096 &  128 & URLLC \\
            \hline
		flow 3  & $256\times 10^3$ & 2048 &  128  & URLLC \\
            \hline
	\end{tabular}
 \begin{tablenotes}
   \item[1] This value already takes into account PD (Propagation Delay).  
  \end{tablenotes}
  \end{threeparttable}

\end{table}

First, we estimate the network bottleneck, which we obtain by calculating the minimum value from the following equations:

\begin{align}
        {R_{1}^{sl,u}}-\rho_{1}^{y(f^{'sl,u})}&={\phi_1^{sl,u} R_{1}}-(\rho_{1}^{2}+\rho_{1}^{3}))=0.5\times0.05\times10^9 - 768\times10^3\\
        {R_{2}^{sl,u}}-\rho_{2}^{y(f^{'sl,u})}&={\phi_2^{sl,u} R_{2}}-(\rho_{2}^{2}+\rho_{2}^{3}))=0.25\times0.1\times10^9 - 768\times10^3\\
        {R_{3}^{sl,u}}-\rho_{3}^{y(f^{'sl,u})}&={\phi_3^{sl,u} R_{3}}-(\rho_{3}^{2}+\rho_{3}^{3}))=0.25\times0.25\times10^9 - 768\times10^3\\
        {R_{4}^{sl,u}}-\rho_{4}^{y(f^{'sl,u})}&={\phi_4^{sl,u} R_{4}}-(\rho_{4}^{2}+\rho_{4}^{3}))=0.125\times0.25\times10^9 - 768\times10^3\\
        {R_{5}^{sl,u}}-\rho_{5}^{y(f^{'sl,u})}&={\phi_5^{sl,u} R_{5}}-(\rho_{5}^{2}+\rho_{5}^{3}))=0.0625\times0.25\times10^9 - 768\times10^3
\end{align}

Moreover, we break apart $ {}^{*}\sigma^{f}_{s}$ (the burst's update term) from (\ref{eq:burst_app}) and we substitute it in (\ref{eq:de2e_app}) for each one of the network nodes, as follows:

\begin{multline}
	D_{e2e}^{f^{'sl,u}}=\frac{1024}{\min\{{(R_{1}^{sl,u}-\rho_{1}^{y(f^{'sl,u})}), (R_{2}^{sl,u}-\rho_{2}^{y(f^{'sl,u})}), (R_{3}^{sl,u}}-\rho_{3}^{y(f^{'sl,u})}), (R_{4}^{sl,u}-\rho_{4}^{y(f^{'sl,u})}),(R_{5}^{sl,u}-\rho_{5}^{y(f^{'sl,u})})\}}+\\
	+T_{1}+\frac{{}^*\sigma_{1}^{2}+{}^*\sigma_{1}^{3}}{R_{1}^{sl,u}}+T_{2}+\frac{{}^*\sigma_{2}^{2}+{}^*\sigma_{2}^{3}}{R_{2}^{sl,u}}+T_{3}+\frac{{}^*\sigma_{3}^{2}+{}^*\sigma_{3}^{3}}{R_{3}^{sl,u}}+T_{4}+\frac{{}^*\sigma_{4}^{2}+{}^*\sigma_{4}^{3}}{R_{4}^{sl,u}}+T_{5}+\frac{{}^*\sigma_{5}^{2}+{}^*\sigma_{5}^{3}}{R_{5}^{sl,u}},
	% \label{eq:de2e_6c}
\end{multline}

\noindent where

\begin{align}
        {}^{*}\sigma^{2}_{1}&=\sigma^{2}=4096,\\
        {}^{*}\sigma^{3}_{1}&=\sigma^{3}=2048,\\ {}^{*}\sigma^{2}_{2}&=\sigma^{2}+\rho^{2}T_{1}=4116.97152,\\ {}^{*}\sigma^{3}_{2}&=\sigma^{3}+\rho^{3}T_{1}=2058.48576,\\
        {}^{*}\sigma^{2}_{3}&=\sigma^{2}+\rho^{2}(T_{1}+T_{2})=4137.94304,\\
        {}^{*}\sigma^{3}_{3}&=\sigma^{3}+\rho^{3}(T_{1}+T_{2})=2068.97152,\\
        {}^{*}\sigma^{2}_{4}&=\sigma^{2}+\rho^{2}(T_{1}+T_{2}+T_{3})=4156.571648,\\
        {}^{*}\sigma^{3}_{4}&=\sigma^{3}+\rho^{3}(T_{1}+T_{2}+T_{3})=2078.285824,\\
        {}^{*}\sigma^{2}_{5}&=\sigma^{2}+\rho^{2}(T_{1}+T_{2}+T_{3}+T_{4})=4171.005952,\\
        {}^{*}\sigma^{3}_{5}&=\sigma^{3}+\rho^{3}(T_{1}+T_{2}+T_{3}+T_{4})=2085.502976,
\end{align}

\begin{multline}
	D_{e2e}^{f^{'sl,u}}=\frac{1024}{(0.25\times0.0625\times10^9 - 768\times10^3)}
	+(40.96+40.96+36.384+28.192+24.096)\times10^{-6}+\\+\frac{{}^*\sigma_{1}^{2}+{}^*\sigma_{1}^{3}}{R_{1}^{sl,u}}+\frac{{}^*\sigma_{2}^{2}+{}^*\sigma_{2}^{3}}{R_{2}^{sl,u}}+\frac{{}^*\sigma_{3}^{2}+{}^*\sigma_{3}^{3}}{R_{3}^{sl,u}}+\frac{{}^*\sigma_{4}^{2}+{}^*\sigma_{4}^{3}}{R_{4}^{sl,u}}+\frac{{}^*\sigma_{5}^{2}+{}^*\sigma_{5}^{3}}{R_{5}^{sl,u}},
	% \label{eq:de2e_6c}
\end{multline}

\begin{multline}
	D_{e2e}^{f^{'sl,u}}=\frac{1024}{14.857\times10^6}
	+170.592\times10^{-6}+\\+\frac{6144}{0.025\times 10^9}+\frac{6175.45728}{0.025\times10^9}+\frac{6206.91456}{0.0625\times10^9}+\frac{6234.857472}{0.03125\times10^9}+\frac{6256.508928}{0.015625\times10^9},
	% \label{eq:de2e_6c}
\end{multline}

\begin{equation}
D_{e2e}^{f^{'sl,u}}=1.43153667431 ms
\end{equation}

\subsection{Parameters for the network topology depicted in Figure \ref{fig:queueingModel} - last update 25.01.2023}

\begin{table}[htb]
	\centering
\begin{threeparttable}
	\caption{Parameters for Simulation with URLLC flows and Bundled Option (D-RAN) as the O-RAN scenario (see subsection \ref{subsection:O-ran}).}
           \label{Tab:Parameters1}
	\begin{tabular}{|c|c|c|}
		\hline
		Parameter & $R$ (Mbps) & $T\tnote{1}$ ($\mu$s) \\
		\hline
		vDU & 150 & $L_{max}*8/150$  \\
		\hline
            eth & 1000 & $L_{max}*8/1000$   \\
		\hline
		ring & 2500 & $L_{max}*8/2500$   \\
		  \hline
		\hline
		Parameter & $\rho$ (bps) & $\sigma$ (bits)\\
            \hline
		flow  & $1024\times 10^3$ & 1024 \\
		\hline
	\end{tabular}
 \begin{tablenotes}
   \item[1] This value is obtained using $T=\frac{L_{max}*8}{R}$. For URLLC, we considered a packet size of $L_{max}$=128 Bytes.  
  \end{tablenotes}
  \end{threeparttable}
\end{table}
\begin{table}[htb]
	\centering
\begin{threeparttable}
	\caption{Parameters for Simulation with URLLC flows and Med/MAcro (C-RAN) as the O-RAN scenario (see subsection \ref{subsection:O-ran}).}
           \label{Tab:Parameters2}

	\begin{tabular}{|c|c|c|}
		\hline
		Parameter & $R$ (Mbps) & $T\tnote{1}$ ($\mu$s) \\
		\hline
		vDU & 1200 & $L_{max}*8/1200$  \\
		\hline
            eth & 8000 & $L_{max}*8/8000$   \\
		\hline
		ring & 20000 & $L_{max}*8/20000$   \\
		  \hline
		\hline
		Parameter & $\rho$ (bps) & $\sigma$ (bits)\\
            \hline
		flow  & $7731\times 10^3$ & 7731 \\
		\hline
	\end{tabular}
 \begin{tablenotes}
   \item[1] This value is obtained using $T=\frac{L_{max}*8}{R}$. For URLLC, we considered a packet size of $L_{max}$=128 Bytes.  
  \end{tablenotes}
  \end{threeparttable}

\end{table}

\begin{figure}[!hb]
    \centering
    \includegraphics[width=3.5in]{Figures/delay_UE_example1.eps}
    \caption{Delay results for the topology depicted in Figure \ref{fig:queueingModel}. For this simulation, a single RU is active. We vary the number of UEs connected to the RU. The red dotted line represents the SLA (application requirement ($<$ 1ms)). Propagation delay is not taken into account in the results plotted in this Figure.}
    \label{fig:delay_UE_example1}
\end{figure}

\subsection{O-RAN scenarios}
\label{subsection:O-ran}

\begin{enumerate}
    \item Bundled Option

RU/DU/CU $\longleftrightarrow$ UPF(s)

\item Small to Mid

RU/DU $\leftarrow$split 2$\rightarrow$CU$\longleftrightarrow$UPF(s)

\item Med/Macro

RU $\leftarrow$split 7.2x$\rightarrow$DU/CU$\longleftrightarrow$UPF(s)

\item Macro

RU $\leftarrow$split 7.2x$\rightarrow$DU$\leftarrow$split 2$\rightarrow$CU$\longleftrightarrow$UPF(s)
\end{enumerate}
